# Supplementary material for: Exploring dependence between categorical variables: benefits and limitations of using variable selection within Bayesian clustering in relation to log-linear modelling with interaction terms
Source: arXiv:1401.7214 source file (2016-01-05)
Supplement: Supplementary file 1 [file SuppInfo_Papathomas_Richardson.pdf]

# Supplemental Material

## On the utility of the Dirichlet process for linear model determination: application to graphical log-linear model determination

Michail Papathomas<sup>1</sup> and Sylvia Richardson<sup>2</sup>

<sup>1</sup> *School of Mathematics and Statistics, University of St Andrews, United Kingdom*

<sup>2</sup> *MRC Biostatistics Unit, Institute of Public Health, Cambridge, United Kingdom*

\* Correspondence to: Michail Papathomas

*The Observatory, University of St Andrews, Buchanan Gardens, St Andrews, Fife, Scotland, UK, KY16 9LZ, michail@mcs.st-and.ac.uk*

### S1. A formal definition of interaction terms in a log-linear model

Denote with  $\mathcal{P}$  the finite set of the  $P$  categorical covariates or factors. The resulting data can be arranged as counts in a  $P$ -way contingency table. A Poisson log-linear interaction model is a generalized linear model where the data are the cell counts of the contingency table. Denote with  $I_p$  the set of levels of factor  $x_p$ . Adopting the notation of Darroch et al. (1980), an individual cell is denoted by  $\mathbf{l} = (l_p, p \in \mathcal{P})$ , where  $l_p$  is an element of  $I_p$ . In other words,  $\mathbf{l}$  is a vector of size  $P$ , with elements that describe the level of each factor. The cell count of  $\mathbf{l}$  is denoted by  $n(\mathbf{l})$ . The cell counts are taken to be independent Poisson variables. The mean  $\mu(\mathbf{l})$  of a certain cell is expanded so that,

$$\mu(\mathbf{l}) = \sum_{a \subseteq \mathcal{P}} \xi_a(\mathbf{l}_a).$$

Here,  $\mathbf{l}_a = (l_p, p \in a)$  indicates a marginal cell defined by the levels of a subset  $a$  of  $\mathcal{P}$ . In the above sum, each term represents parameters  $\xi_a$ , one for each combination of levels of the factors in  $a$ . As pointed out in Dellaportas and Forster (1999), the  $\xi_a$  are equivalent to the parameters commonly used when a specific log-linear model is defined. When  $a = \emptyset$ , the  $\xi_a$  is a constant. When  $|a| = 1$ ,  $\xi_a$  is called a 'main effect'. When  $|a| = m$ ,  $\xi_a$  is an interaction of

order  $m - 1$ . To ensure identifiability, certain  $\xi_a$  parameters are apriori set equal to zero. If the number of individuals is fixed, say equal to  $n$ , the conditional distribution of the cell counts becomes multinomial and a constraint is added to the model to ensure that the total of the cell counts is  $n$ .

## S2. Calculation of the $T_\gamma$ matrices

In this and the next Section, we demonstrate in detail some technical aspects of our methodology. Throughout Sections S2 and S3 we use as a working example the real data analysis presented in Section 5.1 of the main manuscript, where six risk factors for coronary heart disease (CHD) were investigated.

To build the  $T_\gamma^{\text{Real data (CHD)}}$  matrix we follow the algorithm proposed in Section 3.3 of the main manuscript. Before reweighting so that the maximum element is one, we obtain,

$$T_\gamma^{\text{Real data (CHD)}} = \begin{pmatrix} 0 & 721129 & \mathbf{725058} & \mathbf{129703} & \mathbf{504982} & 38648 \\ 0 & 0 & \mathbf{893535} & 143723 & \mathbf{670162} & 46371 \\ 0 & 0 & 0 & 145243 & 672967 & 46277 \\ 0 & 0 & 0 & 0 & \mathbf{111174} & 10221 \\ 0 & 0 & 0 & 0 & 0 & 41739 \end{pmatrix}$$

We reweight and obtain,

$$T_\gamma^{\text{Real data (CHD)}} = \begin{pmatrix} 0 & 0.81 & \mathbf{0.81} & \mathbf{0.14} & \mathbf{0.56} & 0.04 \\ 0 & 0 & \mathbf{1} & 0.16 & \mathbf{0.75} & 0.05 \\ 0 & 0 & 0 & 0.16 & 0.75 & 0.05 \\ 0 & 0 & 0 & 0 & \mathbf{0.12} & 0.01 \\ 0 & 0 & 0 & 0 & 0 & 0.05 \end{pmatrix}$$

### S3. A working example for the selection of candidate edges

Assume the currently accepted model in the reversible jump MCMC chain is ‘ABC+DEF’, and consider the  $\mathbf{T}_\gamma^{\text{Real data (CHD)}}$  matrix.

#### Selecting an edge for possible addition

Elements (1, 4), (1, 5), (1, 6), (2, 4), (2, 5), (2, 6), (3, 4), (3, 5), (3, 6), of matrix  $\mathbf{T}_\gamma^{\text{Real data (CHD)}}$  correspond to edges between the following pairs of factors: (AD), (AE), (AF), (BD), (BE), (BF), (CD), (CE), (CF). As stated at the start of this Section, we assume that the currently accepted model is ‘ABC+DEF’. Therefore, these edges are not part of the currently accepted model, and one of them will become candidate edge for adding to the currently accepted model. The aforementioned elements of  $\mathbf{T}_\gamma^{\text{Real data (CHD)}}$  can be arranged as,

$$\begin{pmatrix} - & - & - & \mathbf{0.14} & \mathbf{0.56} & 0.04 \\ - & - & - & 0.16 & \mathbf{0.75} & 0.05 \\ - & - & - & 0.16 & 0.75 & 0.05 \\ - & - & - & - & - & - \\ - & - & - & - & - & - \\ - & - & - & - & - & - \end{pmatrix}$$

We divide each element with the sum of all nine elements, obtaining,

$$\begin{pmatrix} - & - & - & \mathbf{0.0541} & \mathbf{0.2106} & 0.0161 \\ - & - & - & 0.0599 & \mathbf{0.2795} & 0.0193 \\ - & - & - & 0.0605 & 0.2795 & 0.0193 \\ - & - & - & - & - & - \\ - & - & - & - & - & - \\ - & - & - & - & - & - \end{pmatrix}$$

Now, the elements above add up to one. We sample an edge using them as probabilities associated with each one of the candidate edges. It is then proposed to add the selected edge to the currently accepted graphical model.

#### Selecting an edge for possible removal

Elements (1, 2), (1, 3), (2, 3), (4, 5), (4, 6), (5, 6), of matrix  $\mathbf{T}_\gamma^{\text{Real data (CHD)}}$  correspond to

edges  $(AB)$ ,  $(AC)$ ,  $(BC)$ ,  $(DE)$ ,  $(DF)$ ,  $(EF)$ . These edges form the currently accepted model, and one of them will become a candidate edge for removal. The aforementioned elements of  $\mathbf{T}_\gamma^{\text{Real data (CHD)}}$  can be arranged as,

$$\begin{pmatrix} - & 0.81 & \mathbf{0.81} & - & - & - \\ - & & \mathbf{1} & - & - & - \\ - & - & - & - & - & - \\ - & - & - & - & \mathbf{0.12} & 0.01 \\ - & - & - & - & - & 0.05 \end{pmatrix}$$

To randomly select an edge for possible removal, we divide each element with the sum of all six elements, obtaining,

$$\begin{pmatrix} - & 0.2881 & \mathbf{0.2897} & - & - & - \\ - & - & \mathbf{0.3570} & - & - & - \\ - & - & - & - & - & - \\ - & - & - & - & \mathbf{0.0444} & 0.0041 \\ - & - & - & - & - & 0.0167 \end{pmatrix}$$

Now, the elements above add up to one. We sample an edge using these elements as probabilities associated with each one of the candidate edges. It is then proposed to remove the selected edge from the currently accepted graphical model.

### Selecting two edges to swap

To attempt to swap one edge with another, we select a candidate edge for addition and one for simultaneous removal exactly as described above.

#### S4. Parameter coefficients and design matrices for simulated data

We present the parameter coefficients and design matrices for the five simulated data sets.

##### Simulation 1

$$X_1 = 0.097656 \times \begin{pmatrix} 1 & -1 & -1 & 1 & -1 & 1 & -1 & 1 & 1 & -1 & -1 & -1 & -1 & -1 & 1 & -1 & 1 & 1 & -1 \\ 1 & 1 & -1 & -1 & -1 & 1 & -1 & -1 & 1 & -1 & -1 & -1 & -1 & -1 & 1 & -1 & 1 & 1 & -1 \\ \dots & & & & & & & & & & & & & & & & & & & \\ 1 & 1 & 1 & 1 & 1 & 1 & 1 & 1 & 1 & 1 & 1 & 1 & 1 & 1 & 1 & 1 & 1 & 1 & 1 & 1 \end{pmatrix}$$

$$\theta_1 = (20, -1, 1, -1, 1, -1, 1, -1, 1, -1, 1, -1, 1, -1, 1, -1, 1, -1, 1)$$

.

$$X_2 = 0.097656 \times \begin{pmatrix} 1 & -1 & -1 & 1 & -1 & 1 & -1 & 1 & 1 & -1 & -1 & -1 & -1 & -1 & -1 & 1 & 1 \\ 1 & 1 & -1 & -1 & -1 & 1 & -1 & -1 & 1 & -1 & -1 & -1 & -1 & -1 & -1 & 1 & 1 \\ \dots & & & & & & & & & & & & & & & & & \\ 1 & 1 & 1 & 1 & 1 & 1 & 1 & 1 & 1 & 1 & 1 & 1 & 1 & 1 & 1 & 1 & 1 & 1 & 1 & 1 \end{pmatrix}$$

$$\theta_2 = (20, -1, 1, -1, 1, -1, 1, -1, 1, -1, 1, -1, 1, -1, 1, -1, 1, -1, 1)$$

.

$$X_3 = 0.097656 \times \begin{pmatrix} 1 & -1 & -1 & 1 & -1 & 1 & -1 & 1 & 1 & -1 & -1 & -1 & -1 & -1 & -1 & 1 & 1 \\ 1 & 1 & -1 & -1 & -1 & 1 & -1 & -1 & 1 & -1 & -1 & -1 & -1 & -1 & -1 & 1 & 1 \\ \dots & & & & & & & & & & & & & & & & & \\ 1 & 1 & 1 & 1 & 1 & 1 & 1 & 1 & 1 & 1 & 1 & 1 & 1 & 1 & 1 & 1 & 1 & 1 & 1 & 1 \end{pmatrix}$$

$$\theta_3 = (20, -1, 1, -1, 1, -1, 1, -1, 1, -1, 1, -1, 1, -1, 1, -1, 1, -1, 1)$$

.







•

[illegible]



## S5. Profiles of representative clusters for simulations 1-5 and real data analyses

To build a procedure with an easily interpretable end-product, whilst the rich MCMC output is utilized and uncertainty is accounted for, we adopt a model averaging approach described in Papathomas et al. (2012). One aspect of this approach is the derivation of a specific partition that best represents the variable clustering of the subjects during the MCMC run. We refer to this as the ‘representative partition’. This partition is derived using a similarity matrix that summarizes the partitioning across all iterations using pairwise allocation probabilities (Molitor et al., 2010), in tandem with Partitioning Around Medoids (PAM, Kaufman and Rousseeuw, 2005).

First, to clarify our notation, we give a simple illustrative example. Assume we observe eight categorical covariates,  $x_1, \dots, x_8$ , taking values 0,1 and 2. Suppose the subjects are typically allocated into three sub-populations. A description of a possible profile of the three clusters is seen in Table B0. For each covariate  $x_p$  and each possible observation  $x = 0, 1, 2$ , we consider the 95% credible interval (CI) for the difference between the probability  $\phi_p^c(x)$  of attribute  $x$  in group  $c$ , and the corresponding frequency of  $x_p = x$  in the whole sample. Assume that, with regard to the first group and the first covariate, the CI that corresponds to  $x = 0$  is below zero, whilst the two CIs that correspond to  $x = 1, 2$  are above zero. So, for subjects in the first group, it is less likely to observe 0 at the first covariate, compared to the whole sample, and more likely to observe 1 or 2. We denote this information with the ‘<’ and ‘>’ symbols. We use the ‘0’ symbol when the CI contains zero. In Table S1, where we also provide hypothetical posterior medians for  $\rho_p$ ,  $p = 1, \dots, 8$ , we see the hypothetical structure in the population.

**Table S1:** Cluster profiles in hypothetical simple illustration. The ‘<’ (‘>’) symbol denotes that observation  $x$  of covariate  $x_p$  in cluster  $c$  is more (less) likely compared to the average in the whole sample; otherwise, the ‘0’ symbol is used.

|                    | $x_1$ | $x_2$ | $x_3$ | $x_4$ | $x_5$ | $x_6$ | $x_7$ | $x_8$ |
|--------------------|-------|-------|-------|-------|-------|-------|-------|-------|
| Median( $\rho_p$ ) | 0.8   | 0.8   | 0.8   | 0.9   | 0.9   | 0.9   | 0.1   | 0.1   |
| Group 1            | <>>   | <>>   | <>>   | <<>   | <<>   | <<>   | 000   | 000   |
| Group 2            | < 0 > | < 0 > | < 0 > | ><<   | ><<   | ><<   | 000   | 000   |
| Group 3            | ><<   | ><<   | ><<   | ><<   | ><<   | ><<   | 000   | 000   |

In Table S2, we present results from the flexible clustering simulation analyses using the Dirichlet process. In all simulations, we observe clustering structure that corresponds to simulated interactions, although this correspondence is not present in a clear cut manner and does not

help with untangling the different interactions. For simulation 1, three clusters were highlighted in the output summary. Clusters 1 and 2 correspond to the simulated ‘ABCD’ and ‘HIJ’ interactions. The posterior median for the selection probability for ‘C’ is comparable to the medians of other important covariates, however ‘C’ does not appear to contribute to the formation of the cluster profiles as strongly as the other important covariates. Cluster 3 clearly corresponds to the presence of the simulated ‘HIJ’ interaction. For simulation 2, five clusters were highlighted in the output. Clusters 2-5 seem to correspond to the ‘ABCD’ and ‘AFG’ interactions. Two clusters were highlighted in simulation 3. It is interesting to note that their profiles seem to correspond to the ‘ABCD’ and ‘AFG’ interactions, whilst the ‘HIJ’ interaction is not prominent. However, the posterior selection medians for ‘H’, ‘I’ and ‘J’ are as high as the posterior medians of the other important covariates, in accordance with the simulation mechanism. With regard to the fourth simulated data set, the clustering algorithm, after adopting a sparse prior, detected that the last 14 variables are not important for the structure in the data, with  $E(\rho_p) < 0.0045, p = 7, \dots, 20$ , in accordance with the simulation mechanism. In Table S2, we present results from the flexible clustering analysis in relation to the first six covariates. Six clusters comprise the representative partition.

In all simulations, we observe clustering structure that corresponds to the simulated interactions, although this correspondence is not present in a clear cut manner and is not helpful with untangling the different interactions.

In Table S3, we present the covariate profiles of the representative clusters created with the Bayesian partitioning analysis, for the first real data illustration. The subjects are divided in two clusters, and it is not straightforward to disentangle the linear model interactions that are present from the cluster profiles. In Table S3, we also present the profiles of the representative clusters created with the Bayesian partitioning analysis, for the second real data illustration. The subjects are typically divided in two clusters which correspond to the ‘DEF’ interaction.

The representative partitions presented here are derived from the similarity matrix using Partitioning Around Medoids (PAM), a choice we made due to PAM’s stable behaviour in various studies we have undertaken. Another equally valid approach for converting the information in the similarity matrix into a representative partition could be based on a least squares argument (Dahl, 2006). Alternatively, one may choose to use a dendrogram. These three approaches will

often result in different representative partitions. Such instability means that we should not place too much importance on the interpretation of the output presented here.

**Table S2:** Cluster profiles for the five simulations. In parenthesis the number of subjects typically allocated to each group. All posterior median selection probabilities for the remaining 14 covariates in Simulation 4 were equal to zero. Posterior median selection probabilities for the remaining 92 covariates in Simulation 5 were either equal to zero or smaller than 0.01

| Simulation 1       |      |       |      |      |      |      |      |      |      |      |
|--------------------|------|-------|------|------|------|------|------|------|------|------|
|                    | A    | B     | C    | D    | E    | F    | G    | H    | I    | J    |
| Median( $\rho_p$ ) | 0.36 | 0.78  | 0.32 | 0.75 | 0.06 | 0.05 | 0.00 | 0.48 | 0.57 | 0.50 |
| Group 1 (5465)     | ><   | <>    | 00   | <>   | 00   | 00   | 00   | ><   | ><   | <>   |
| Group 2 (3159)     | <>   | ><    | 00   | ><   | 00   | 00   | 00   | ><   | <>   | ><   |
| Group 3 (1376)     | 00   | ><    | 00   | 00   | 00   | 00   | 00   | <>   | <>   | <>   |
| Simulation 2       |      |       |      |      |      |      |      |      |      |      |
|                    | A    | B     | C    | D    | E    | F    | G    | H    | I    | J    |
| Median( $\rho_p$ ) | 0.63 | 0.38  | 0.35 | 0.53 | 0.00 | 0.50 | 0.51 | 0.16 | 0.07 | 0.09 |
| Group 1 (1153)     | 00   | 00    | 00   | 00   | 00   | ><   | ><   | 00   | 00   | 00   |
| Group 2 (1926)     | <>   | ><    | 00   | ><   | 00   | ><   | ><   | 00   | 00   | 00   |
| Group 3 (2031)     | <>   | <>    | ><   | ><   | 00   | ><   | ><   | 00   | 00   | 00   |
| Group 4 (2466)     | <>   | ><    | <>   | <>   | 00   | ><   | ><   | 00   | 00   | 00   |
| Group 5 (2424)     | ><   | <>    | 00   | <>   | 00   | <>   | <>   | 00   | 00   | 00   |
| Simulation 3       |      |       |      |      |      |      |      |      |      |      |
|                    | A    | B     | C    | D    | E    | F    | G    | H    | I    | J    |
| Median( $\rho_p$ ) | 0.38 | 0.50  | 0.30 | 0.54 | 0.07 | 0.34 | 0.49 | 0.41 | 0.43 | 0.66 |
| Group 1 (7676)     | <>   | ><    | 00   | ><   | 00   | ><   | ><   | 00   | 00   | 00   |
| Group 2 (2324)     | ><   | <>    | 00   | <>   | 00   | <>   | <>   | 00   | 00   | 00   |
| Simulation 4       |      |       |      |      |      |      |      |      |      |      |
|                    | A    | B     | C    | D    | E    | F    |      |      |      |      |
| Median( $\rho_p$ ) | 0.96 | 0.85  | 0.95 | 0.59 | 0.71 | 0.55 |      |      |      |      |
| Group 1 (3028)     | ><>  | ><>   | ><>  | ><>  | ><>  | ><>  |      |      |      |      |
| Group 2 (320)      | 000  | <><   | <><  | <> 0 | <> 0 | 0 >< |      |      |      |      |
| Group 3 (739)      | ><>  | >< 0  | ><>  | <><  | <><  | <><  |      |      |      |      |
| Group 4 (215)      | <><  | <><   | <><  | <><  | <><  | <><  |      |      |      |      |
| Group 5 (326)      | <><  | <><   | 00 > | 000  | 0 >< | 0 >< |      |      |      |      |
| Group 6 (372)      | <><  | 0 > 0 | <><  | <> 0 | 0 <> | 0 >< |      |      |      |      |
| Simulation 5       |      |       |      |      |      |      |      |      |      |      |
|                    | A    | B     | C    | D    | E    | F    | G    | H    |      |      |
| Median( $\rho_p$ ) | 0.96 | 0.95  | 0.97 | 0.93 | 0.97 | 0.96 | 0.97 | 0.96 |      |      |
| Group 1 (4036)     | ><   | <>    | <>   | <>   | <>   | ><   | <>   | <>   |      |      |
| Group 2 (3813)     | ><   | <>    | <>   | <>   | ><   | <>   | ><   | ><   |      |      |
| Group 3 (399)      | ><   | 00    | <>   | ><   | <>   | ><   | ><   | <>   |      |      |
| Group 4 (720)      | <>   | ><    | ><   | ><   | <>   | ><   | <>   | <>   |      |      |
| Group 5 (902)      | <>   | ><    | ><   | ><   | ><   | <>   | ><   | ><   |      |      |
| Group 5 (130)      | <>   | ><    | ><   | ><   | ><   | <>   | ><   | <>   |      |      |

**Table S3:** Cluster profiles for the real data illustrations. In parenthesis the number of subjects typically allocated to each group.

| Edwards and Havranek data (CHD) |               |               |               |         |         |             |
|---------------------------------|---------------|---------------|---------------|---------|---------|-------------|
|                                 | A             | B             | C             | D       | E       | F           |
| Median( $\rho_p$ )              | 0.86          | 0.92          | 0.94          | 0.26    | 0.81    | 0.10        |
| Group 1 (900)                   | ><            | <>            | ><            | 00      | <>      | 00          |
| Group 2 (941)                   | <>            | ><            | <>            | 00      | ><      | 00          |
| Genetic-environmental data (GE) |               |               |               |         |         |             |
|                                 | rs8034191 (A) | rs4324798 (B) | rs1950081 (C) | age (D) | sex (E) | smoking (F) |
| Median( $\rho_p$ )              | 0.01          | 0.00          | 0.10          | 0.92    | 0.82    | 0.85        |
| Group 1 (2222)                  | 00            | 00            | 00            | ><      | ><      | <>          |
| Group 2 (2059)                  | 00            | 00            | 00            | <>      | <>      | ><          |

## **S6. Rate of accumulated mass of posterior model probability for Simulations 1,2 and 3**

Figures S1,S2 and S3 show the rate of accumulated posterior model probability for Simulations 1,2 and 3 respectively, with respect to the top ten models. We run four replications for each analysis, averaging over the results. The analyses are based on 110000 iterations of the reversible jump MCMC sampler, thinned to 11000 iterations. The top ten models and associated posterior probabilities were calculated using the search algorithm that combines PDV and the cluster specific approach in a balanced manner. We see that this algorithm performs very well in Simulation 1, and also in Simulation 3. It is not performing as well for Simulation 2, although differences in Simulations 2 and 3 are not very pronounced. The PDV algorithm performs worse than the three other algorithms that employ cluster specific information, over the first 2000 iterations or so. As a note of caution, we must stress that the limited number of replications (4) for each analysis, suggests that increased variability is associated with the information presented in Figures S1,S2 and S3.

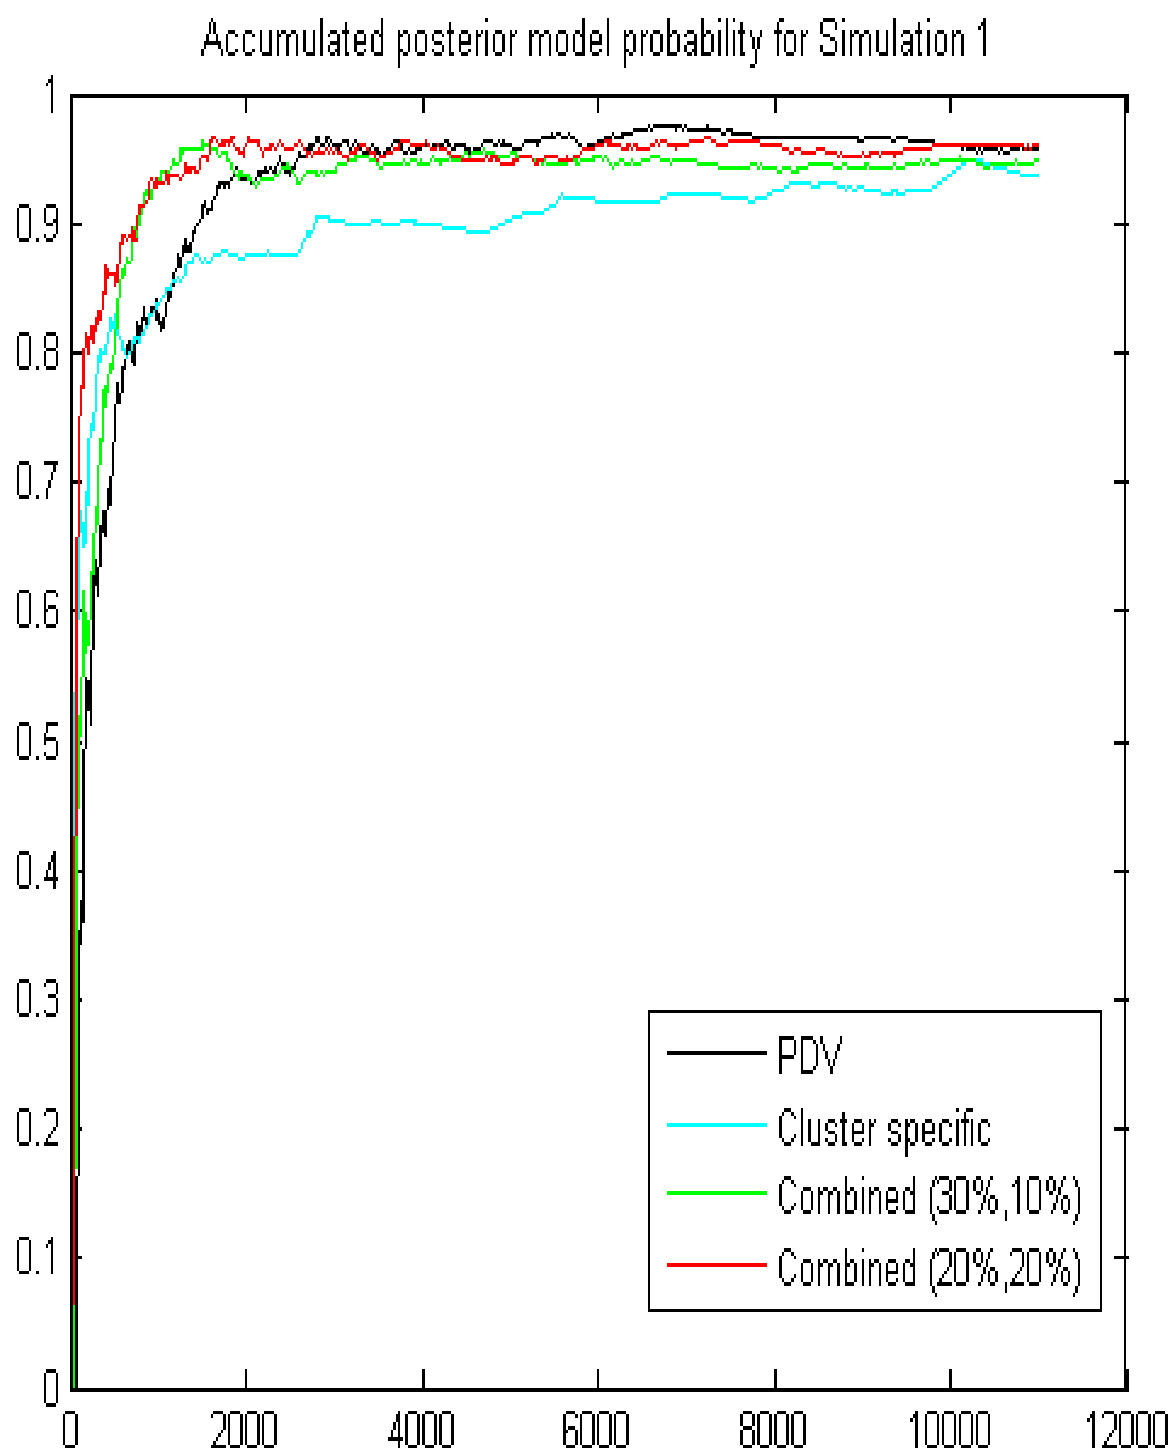

Figure S1: Rate of accumulated posterior model probability for Simulation 1, based on 110000 iterations, thinned to 11000 iterations.

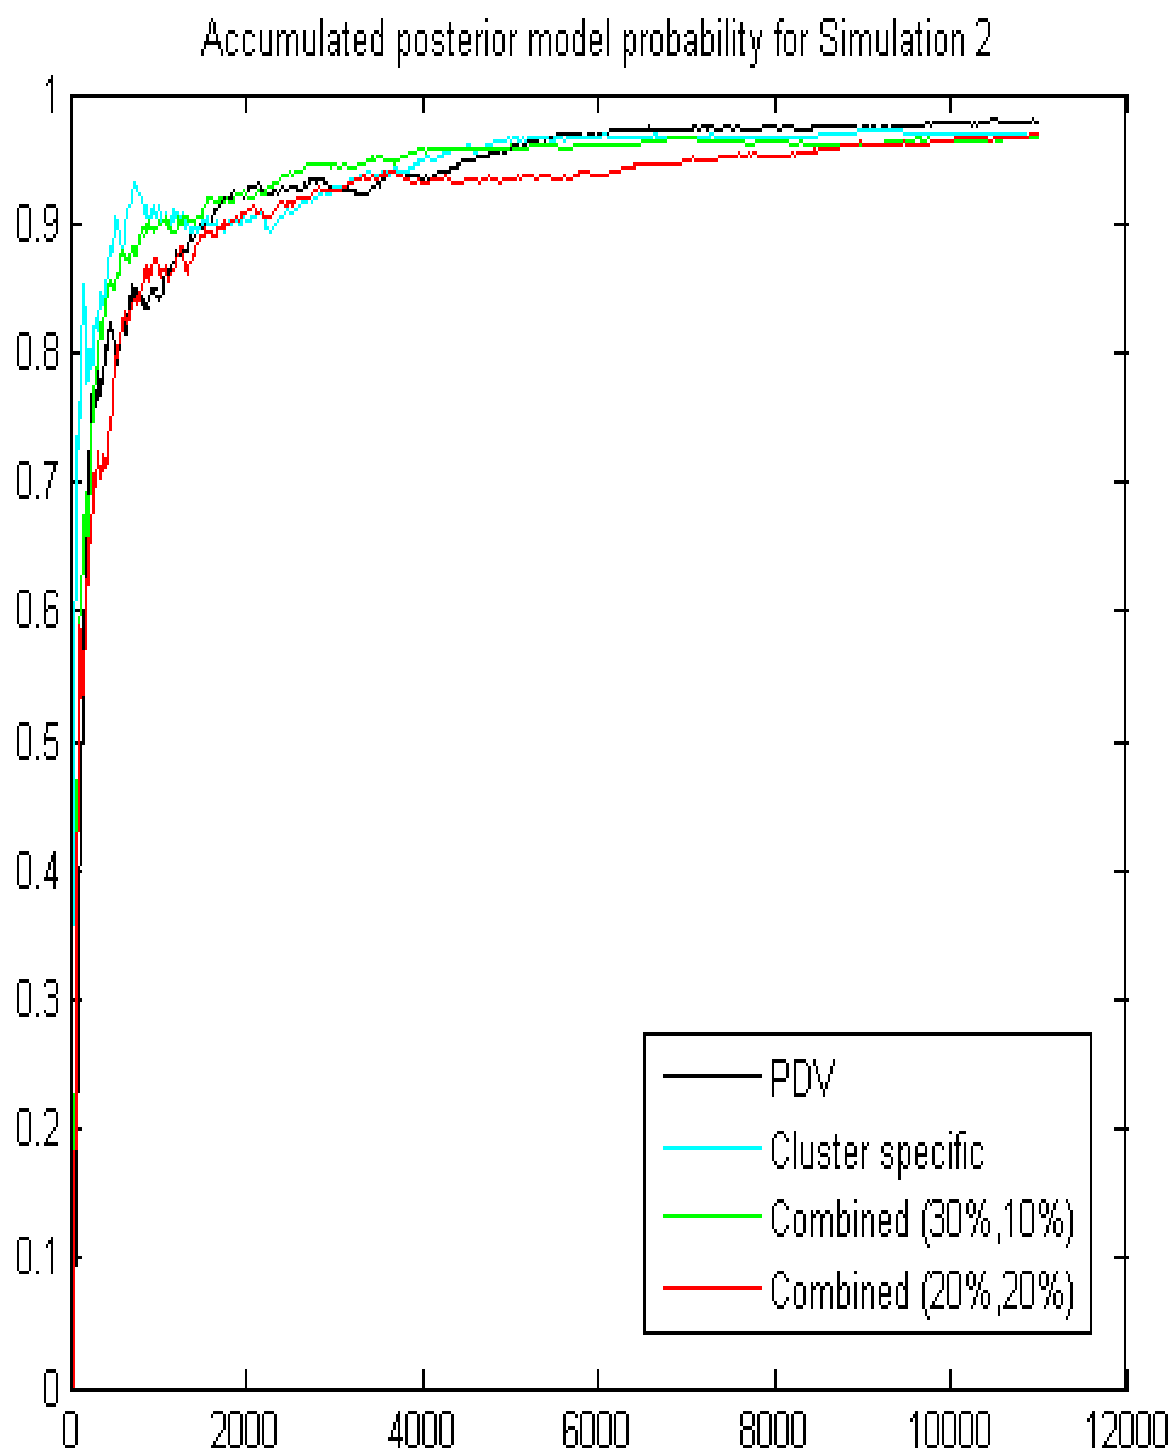

Figure S2: Rate of accumulated posterior model probability for Simulation 2, based on 110000 iterations, thinned to 11000 iterations.

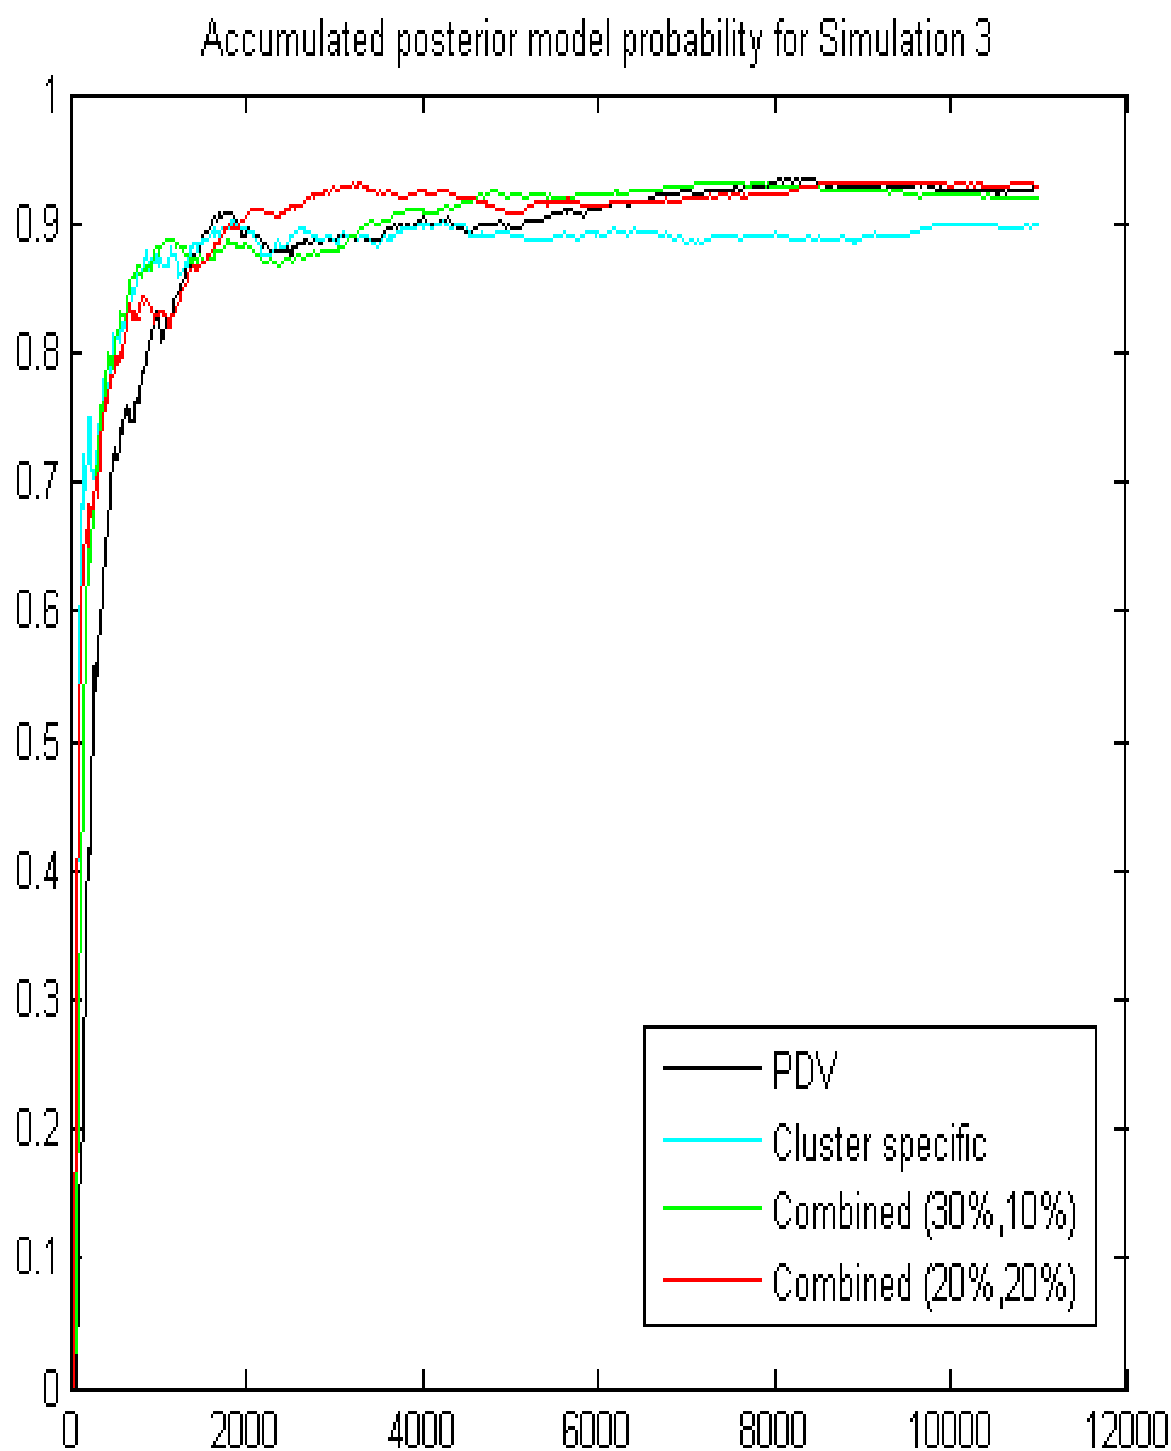

Figure S3: Rate of accumulated posterior model probability for Simulation 3, based on 110000 iterations, thinned to 11000 iterations.

## Reference

- Darroch, J.N., Lauritzen, S.L. & Speed, T.P. (1980). Markov fields and log-linear interaction models for contingency tables. *The Annals of Statistics* **8**, 522-539.
- Dellaportas, P. & Forster, J.J. (1999). Markov chain Monte Carlo model determination for hierarchical and graphical log-linear models. *Biometrika* **86**, 615-633.
- Kaufman, L., Rousseeuw, P.J. (2005). Finding Groups in Data: An Introduction to Cluster Analysis. Wiley Series in Probability and Mathematical Statistics. Hoboken, NJ, Wiley-Interscience.
- Papathomas, M., Molitor, J., Hoggart, C., Hastie, D. & Richardson, S. (2012). Exploring data from genetic association studies using Bayesian variable selection and the Dirichlet process: application to searching for gene-gene patterns. *Genet. Epidemiol.* **36**, 663-674.
